# Supplementary material for: Interpretable Representations in Explainable AI: From Theory to Practice
Source: arXiv:2008.07007 source file (2024-04-26)
Supplement: Supplementary file 1 [file ijcai20-appendix-ols.pdf]

## C Analytical Solution to OLS for Binary Interpretable Representations of Tabular Data

Linear models can be used to quantify importance of interpretable concepts for black-box predictions [Friedman *et al.*, 2008; Ribeiro *et al.*, 2016]. However, for some binary interpretable domains, such an approach is inherently flawed. In this appendix, we show how the interpretable concept importance measured by coefficients of a linear model may be deceiving. This phenomenon is particularly prominent for tabular data transformed into the binary interpretable representation introduced in Section 3. The insights stemming from our analysis can be used to manipulate surrogate explanations, e.g., those produced with LIME [Ribeiro *et al.*, 2016], by using specially crafted, yet perfectly valid, IR discretisation and data sample.

Our results are based on the analytical solution to unweighted ( $\Theta$ ) and weighted ( $\Theta_{\mathbf{W}}$ ) OLS outlined in the equations below, where  $\mathbf{X}$  is the binary interpretable representation data matrix,  $\mathbf{W}$  is the weight matrix, and  $\mathbf{y}$  is the black-box predictions vector. In our analysis, we assume that the black box is a probabilistic classifier, in which case  $\mathbf{y}$  holds probabilities of the explained class, however a similar line of reasoning applies to regressors and crisp classifiers. In the latter case, the predictions are assumed to be 1 if they are the same as the class assigned to the explained instance by the black box, and 0 for any other class. Modelling  $\mathbf{y}$  in such a way is equivalent to generating one-vs-rest explanations of probabilistic black boxes since they only model probabilities of the explained class. Nonetheless, both approaches measure the importance of interpretable concepts – using the coefficients of linear models – for a selected class when tasked with telling it apart from the other classes.

$$\begin{aligned}\Theta &= (\mathbf{X}^T \mathbf{X})^{-1} \mathbf{X}^T \mathbf{y} \\ \Theta_{\mathbf{W}} &= (\mathbf{X}^T \mathbf{W} \mathbf{X})^{-1} \mathbf{X}^T \mathbf{W} \mathbf{y}\end{aligned}$$

In the interest of brevity and readability, we analyse tabular data with two numerical features – akin to the example shown in Figure 6 – but our findings generalise to an arbitrary number of attributes that are both categorical and numerical. In a generic setting, for  $n$  features there will be  $n$  binary concepts with  $2^n$  unique encodings (cardinality) in the interpretable representation. If additionally we choose to model the intercept of the linear model, a phantom all-1 column vector is inserted at the front of the data matrix  $\mathbf{X}$ . Therefore, the  $\mathbf{X}^T \mathbf{X}$  and  $\mathbf{X}^T \mathbf{W} \mathbf{X}$  components of  $\Theta$  and  $\Theta_{\mathbf{W}}$  respectively are square matrices of  $n \times n$  shape sans the intercept or  $(n+1) \times (n+1)$  when the intercept is modelled.

Figure 6 depicts a simplistic view of sampling for two numerical features with just one data point in each hyper-rectangle, but in reality, we should expect their large number since it allows to better approximate the behaviour of the black box, especially when the number of features is high. In this particular case, the binary interpretable representation data matrix  $\mathbf{X}$  – with the first column (red) inserted for modelling the intercept and the remaining columns (blue) representing the binary data – is:

$$\mathbf{X} = \begin{bmatrix} 1 & 1 & 1 \\ 1 & 1 & 0 \\ 1 & 1 & 0 \\ 1 & 0 & 1 \\ 1 & 0 & 1 \\ 1 & 0 & 0 \\ 1 & 0 & 0 \\ 1 & 0 & 0 \\ 1 & 0 & 0 \end{bmatrix},$$

which gives:

$$\mathbf{X}^T \mathbf{X} = \begin{bmatrix} 1 & 1 & 1 & 1 & 1 & 1 & 1 & 1 & 1 \\ 1 & 1 & 1 & 0 & 0 & 0 & 0 & 0 & 0 \\ 1 & 0 & 0 & 1 & 1 & 0 & 0 & 0 & 0 \end{bmatrix} \times \begin{bmatrix} 1 & 1 & 1 \\ 1 & 1 & 0 \\ 1 & 1 & 0 \\ 1 & 0 & 1 \\ 1 & 0 & 1 \\ 1 & 0 & 0 \\ 1 & 0 & 0 \\ 1 & 0 & 0 \\ 1 & 0 & 0 \end{bmatrix} = \begin{bmatrix} 9 & 3 & 3 \\ 3 & 3 & 1 \\ 3 & 1 & 3 \end{bmatrix}.$$

Since some of the hyper-rectangles are merged when transitioning from the discrete into the binary interpretable representation,  $\mathbf{X}$  contains duplicated rows. The influence of this phenomenon is magnified even more when multiple data points are sampled within a single hyper-rectangle. Without loss of generality, we can use the *weighted* variant of OLS, with the data set  $\mathbf{X}$  containing only one copy of each unique binary data point and the weights corresponding to their counts. In this case:

$$\mathbf{X} = \begin{bmatrix} 1 & 1 & 1 \\ 1 & 1 & 0 \\ 1 & 0 & 1 \\ 1 & 0 & 0 \end{bmatrix} \quad \text{and} \quad \mathbf{W} = \begin{bmatrix} w_{11} & 0 & 0 & 0 \\ 0 & w_{10} & 0 & 0 \\ 0 & 0 & w_{01} & 0 \\ 0 & 0 & 0 & w_{00} \end{bmatrix},$$

where  $w_{ij}$  is the count of data points residing in all of the hyper-rectangles that are assigned the  $(i, j)$  coordinates in the binary interpretable representation – see the  $(x^*, y^*)$  coordinates in Figure 6 for reference. Therefore, for an arbitrary number of data points with two numerical features when modelling the intercept:

$$\begin{aligned}
\mathbf{X}^T \mathbf{W} \mathbf{X} &= \begin{bmatrix} 1 & 1 & 1 & 1 \\ 1 & 1 & 0 & 0 \\ 1 & 0 & 1 & 0 \end{bmatrix} \times \begin{bmatrix} w_{11} & 0 & 0 & 0 \\ 0 & w_{10} & 0 & 0 \\ 0 & 0 & w_{01} & 0 \\ 0 & 0 & 0 & w_{00} \end{bmatrix} \times \begin{bmatrix} 1 & 1 & 1 \\ 1 & 1 & 0 \\ 1 & 0 & 1 \\ 1 & 0 & 0 \end{bmatrix} \\
&= \begin{bmatrix} w_{11} & w_{10} & w_{01} & w_{00} \\ w_{11} & w_{10} & 0 & 0 \\ w_{11} & 0 & w_{01} & 0 \end{bmatrix} \times \begin{bmatrix} 1 & 1 & 1 \\ 1 & 1 & 0 \\ 1 & 0 & 1 \\ 1 & 0 & 0 \end{bmatrix} \\
&= \begin{bmatrix} \sum w_{ij} & w_{11} + w_{10} & w_{11} + w_{01} \\ w_{11} + w_{10} & w_{11} + w_{10} & w_{11} \\ w_{11} + w_{01} & w_{11} & w_{11} + w_{01} \end{bmatrix}.
\end{aligned}$$

For the example in Figure 6 – where  $w_{11} = 1$ ,  $w_{10} = 2$ ,  $w_{01} = 2$  and  $w_{00} = 4$  – a calculation for the weighted variant agrees with the previous result computed directly for  $\mathbf{X}^T \mathbf{X}$ .

Next, we analyse the second component of the  $\Theta_{\mathbf{W}}$  formula:

$$\begin{aligned}
\mathbf{X}^T \mathbf{W} \mathbf{y} &= \begin{bmatrix} 1 & 1 & 1 & 1 \\ 1 & 1 & 0 & 0 \\ 1 & 0 & 1 & 0 \end{bmatrix} \times \begin{bmatrix} w_{11} & 0 & 0 & 0 \\ 0 & w_{10} & 0 & 0 \\ 0 & 0 & w_{01} & 0 \\ 0 & 0 & 0 & w_{00} \end{bmatrix} \times \begin{bmatrix} y_{11} \\ y_{10} \\ y_{01} \\ y_{00} \end{bmatrix} \\
&= \begin{bmatrix} w_{11} & w_{10} & w_{01} & w_{00} \\ w_{11} & w_{10} & 0 & 0 \\ w_{11} & 0 & w_{01} & 0 \end{bmatrix} \times \begin{bmatrix} y_{11} \\ y_{10} \\ y_{01} \\ y_{00} \end{bmatrix} \\
&= \begin{bmatrix} \sum w_{ij} y_{ij} \\ w_{11} y_{11} + w_{10} y_{10} \\ w_{11} y_{11} + w_{01} y_{01} \end{bmatrix}.
\end{aligned}$$

However, this formulation assumes that all of the data points that share the same coordinates in the binary interpretable representation have the same label  $y$ . To allow multiple copies of the same data point with distinct labels, we generalise this result by going back to  $\Theta$ , which is the solution to the classic OLS. This approach is valid since the weighted OLS for which the weights represent the count of each unique data point is equivalent to the classic OLS for a data set whose instances are duplicated according to the counts given by the corresponding weights.

Let us denote  $f : \mathcal{X} \rightarrow \mathcal{Y}$  as the black-box model and  $IR : \mathcal{X} \rightarrow \mathcal{X}^*$  as the transformation function from tabular data  $\mathcal{X}$  into their binary interpretable representation  $\mathcal{X}^*$ . Let us further define  $\mathcal{W}_{ij} = \{x \in \mathbf{X} : IR(x) = (i, j)\}$  as the set of all the data points that are assigned the same interpretable binary representation  $(i, j)$ , and  $\mathcal{W} = \mathbf{X}$  as the set of all the data points. Now, recall that  $w_{ij}$  is the count of data points whose binary interpretable representation is  $(i, j)$ , therefore  $|\mathcal{W}_{ij}| = w_{ij}$  and  $|\mathcal{W}| = \sum w_{ij}$ . Without loss of generality, we can reformulate the  $\mathbf{X}^T \mathbf{W} \mathbf{y}$  part of the  $\Theta_{\mathbf{W}}$  equation as  $\mathbf{X}^T \mathbf{y}$  in order to sum over all of the black-box predictions for their respective hyper-rectangles:

$$\mathbf{X}^T \mathbf{y} = \begin{bmatrix} \sum w_{ij} y_{ij} \\ w_{11} y_{11} + w_{10} y_{10} \\ w_{11} y_{11} + w_{01} y_{01} \end{bmatrix} = \begin{bmatrix} \sum_{i \in \mathcal{W}} y_i \\ \sum_{i \in \mathcal{W}_{11} \cup \mathcal{W}_{10}} y_i \\ \sum_{i \in \mathcal{W}_{11} \cup \mathcal{W}_{01}} y_i \end{bmatrix}.$$

This step allows us to relax the assumption of duplicated labels without loss of generality, hence not impose restrictions on whether the black box is probabilistic and whether the discrete representation has perfect fidelity with respect to the black box.

Finally, to better understand the meaning of importance-based explanations, we reformulate the sum of black-box predictions

into their average:

$$\begin{aligned}
\mathbf{X}^T \mathbf{y} &= \begin{bmatrix} \sum_{i \in \mathcal{W}} y_i \\ \sum_{i \in \mathcal{W}_{11} \cup \mathcal{W}_{10}} y_i \\ \sum_{i \in \mathcal{W}_{11} \cup \mathcal{W}_{01}} y_i \end{bmatrix} = \begin{bmatrix} \sum_{i \in \mathcal{W}} y_i / \sum w_{ij} * \sum w_{ij} \\ \sum_{i \in \mathcal{W}_{11} \cup \mathcal{W}_{10}} y_i / (w_{11} + w_{10}) * (w_{11} + w_{10}) \\ \sum_{i \in \mathcal{W}_{11} \cup \mathcal{W}_{01}} y_i / (w_{11} + w_{01}) * (w_{11} + w_{01}) \end{bmatrix} = \begin{bmatrix} \bar{y}_{\mathcal{W}} * \sum w_{ij} \\ \bar{y}_{\mathcal{W}_{11} \cup \mathcal{W}_{10}} * (w_{11} + w_{10}) \\ \bar{y}_{\mathcal{W}_{11} \cup \mathcal{W}_{01}} * (w_{11} + w_{01}) \end{bmatrix} \\
&= \begin{bmatrix} 1 & 0 & 0 \\ 0 & 1 & 0 \\ 0 & 0 & 1 \end{bmatrix} \times \begin{bmatrix} \bar{y}_{\mathcal{W}} * \sum w_{ij} \\ \bar{y}_{\mathcal{W}_{11} \cup \mathcal{W}_{10}} * (w_{11} + w_{10}) \\ \bar{y}_{\mathcal{W}_{11} \cup \mathcal{W}_{01}} * (w_{11} + w_{01}) \end{bmatrix} \\
&= \begin{bmatrix} \sum w_{ij} & 0 & 0 \\ 0 & w_{11} + w_{10} & 0 \\ 0 & 0 & w_{11} + w_{01} \end{bmatrix} \times \begin{bmatrix} \bar{y}_{\mathcal{W}} \\ \bar{y}_{\mathcal{W}_{11} \cup \mathcal{W}_{10}} \\ \bar{y}_{\mathcal{W}_{11} \cup \mathcal{W}_{01}} \end{bmatrix},
\end{aligned}$$

and combine this result with  $\mathbf{X}^T \mathbf{W} \mathbf{X}$ :

$$\begin{aligned}
&\begin{bmatrix} \sum w_{ij} & w_{11} + w_{10} & w_{11} + w_{01} \\ w_{11} + w_{10} & w_{11} + w_{10} & w_{11} \\ w_{11} + w_{01} & w_{11} & w_{11} + w_{01} \end{bmatrix}^{-1} \times \begin{bmatrix} \sum w_{ij} & 0 & 0 \\ 0 & w_{11} + w_{10} & 0 \\ 0 & 0 & w_{11} + w_{01} \end{bmatrix} \times \begin{bmatrix} \bar{y}_{\mathcal{W}} \\ \bar{y}_{\mathcal{W}_{11} \cup \mathcal{W}_{10}} \\ \bar{y}_{\mathcal{W}_{11} \cup \mathcal{W}_{01}} \end{bmatrix} \\
&= \begin{bmatrix} \sum w_{ij} & w_{11} + w_{10} & w_{11} + w_{01} \\ w_{11} + w_{10} & w_{11} + w_{10} & w_{11} \\ w_{11} + w_{01} & w_{11} & w_{11} + w_{01} \end{bmatrix}^{-1} \times \begin{bmatrix} \frac{1}{\sum w_{ij}} & 0 & 0 \\ 0 & \frac{1}{w_{11} + w_{10}} & 0 \\ 0 & 0 & \frac{1}{w_{11} + w_{01}} \end{bmatrix}^{-1} \times \begin{bmatrix} \bar{y}_{\mathcal{W}} \\ \bar{y}_{\mathcal{W}_{11} \cup \mathcal{W}_{10}} \\ \bar{y}_{\mathcal{W}_{11} \cup \mathcal{W}_{01}} \end{bmatrix} \\
&= \left( \begin{bmatrix} \frac{1}{\sum w_{ij}} & 0 & 0 \\ 0 & \frac{1}{w_{11} + w_{10}} & 0 \\ 0 & 0 & \frac{1}{w_{11} + w_{01}} \end{bmatrix} \times \begin{bmatrix} \sum w_{ij} & w_{11} + w_{10} & w_{11} + w_{01} \\ w_{11} + w_{10} & w_{11} + w_{10} & w_{11} \\ w_{11} + w_{01} & w_{11} & w_{11} + w_{01} \end{bmatrix} \right)^{-1} \times \begin{bmatrix} \bar{y}_{\mathcal{W}} \\ \bar{y}_{\mathcal{W}_{11} \cup \mathcal{W}_{10}} \\ \bar{y}_{\mathcal{W}_{11} \cup \mathcal{W}_{01}} \end{bmatrix} \\
&= \begin{bmatrix} 1 & \frac{w_{11} + w_{10}}{\sum w_{ij}} & \frac{w_{11} + w_{01}}{\sum w_{ij}} \\ 1 & 1 & \frac{w_{11}}{w_{11} + w_{10}} \\ 1 & \frac{w_{11}}{w_{11} + w_{10}} & 1 \end{bmatrix}^{-1} \times \begin{bmatrix} \bar{y}_{\mathcal{W}} \\ \bar{y}_{\mathcal{W}_{11} \cup \mathcal{W}_{10}} \\ \bar{y}_{\mathcal{W}_{11} \cup \mathcal{W}_{01}} \end{bmatrix}.
\end{aligned}$$

This outcome allows us to draw conclusions about the meaning of interpretable concept importance given by the coefficients of a surrogate linear model when the intercept is modelled (red & blue) and without it (blue). In particular, the importance of interpretable concepts is *solely* based on:

- **the proportion determined by the number of the data points** residing in the explained hyper-rectangle ( $\mathcal{W}_{11}$ ) divided by the hyper-rectangles aligned with the explained hyper-rectangle along every axis:  $\mathcal{W}_{11} \cup \mathcal{W}_{10}$  for the first feature and  $\mathcal{W}_{11} \cup \mathcal{W}_{01}$  for the second; and
- **the average value predicted** in the latter two subspaces –  $\mathcal{W}_{11} \cup \mathcal{W}_{10}$  and  $\mathcal{W}_{11} \cup \mathcal{W}_{01}$  – by the black box (scaled appropriately when the intercept is modelled).

For example, consider Figure 9 where  $x_1^*$  denotes the first binary interpretable feature and  $x_2^*$  the second. In this case,  $\mathcal{W}_{11}$  is the yellow hyper-rectangle;  $\mathcal{W}_{11} \cup \mathcal{W}_{10}$  is the union of the yellow and green hyper-rectangles; and  $\mathcal{W}_{11} \cup \mathcal{W}_{01}$  is the combination of yellow and blue hyper-rectangles. Finally,  $\bar{y}_{\mathcal{W}_{11} \cup \mathcal{W}_{10}}$  is the average prediction in the vertical green&yellow segment, and  $\bar{y}_{\mathcal{W}_{11} \cup \mathcal{W}_{01}}$  is the average prediction in the horizontal blue&yellow stripe.

The intercept value is additionally determined by:

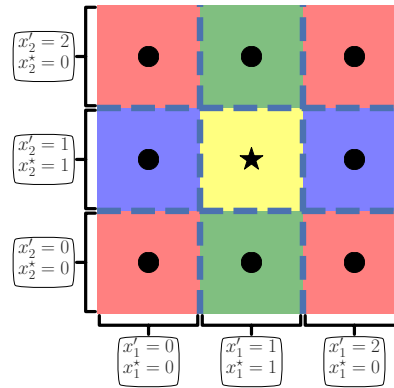

Figure 9: Example of discrete  $(x'_1, x'_2)$  and binary interpretable  $(x_1^*, x_2^*)$  representations of tabular data.  $\star$  represents the explained instance.

- *the proportion* given by the number of data points in the hyper-rectangles aligned with the explained hyper-rectangle along every axis divided by the total number of data points; and
- *the average* value predicted by the black box for all the data points.

Intuitively, the instances not aligned with the explained hyper-rectangle – red blocks in Figure 9 – are assigned the  $(0, 0)$  coordinates in the binary interpretable representation, therefore they cannot contribute to the feature coefficients of a linear model, just the intercept. This can be easily seen with  $g(\mathbf{x}; \Theta) = \sum_{i=0}^n \Theta_i x_i$  formula, where  $x_0 = 1$  is the phantom feature and the remaining data features  $x_1, \dots, x_n$  are 0.

An important insight uncovered by these results is **partial irrelevance of the discretisation quality** given a fixed number of data points placed in the identified collections of hyper-rectangles. Using this property, we can manipulate the explanation by altering the number of data points in relevant partitions, with the discretisation faithfulness having relatively small influence. For example, consider the two discretisations depicted earlier in Figure 5, assuming that the explained hyper-rectangle is  $(x', y') = (1, 1)$  for both sub-plots and that the  $(x', y') = (1, 0)$  and  $(x', y') = (1, 1)$  partitions in Figure 5b have *three* additional data points each. In this case, when modelling the importance of interpretable components without the intercept, the only difference between these two sub-plots are the predictions of the instances placed in the expanded hyper-rectangles, i.e.,  $(x', y') = (1, 0)$  and  $(x', y') = (1, 1)$ , since:

**Figure 5a**  $w_{11} = 4$ ,  $w_{01} = 4 + 4 = 8$  and  $w_{10} = 4$ , leading to  $\frac{w_{11}}{w_{11}+w_{10}} = \frac{4}{4+4} = \frac{1}{2}$  and  $\frac{w_{11}}{w_{11}+w_{01}} = \frac{4}{4+8} = \frac{1}{3}$ ; and

**Figure 5b**  $w_{11} = 2 + 3 = 5$ ,  $w_{01} = 4 + 4 + 2 = 10$  and  $w_{10} = 2 + 3 = 5$ , leading to  $\frac{w_{11}}{w_{11}+w_{10}} = \frac{5}{5+5} = \frac{1}{2}$  and  $\frac{w_{11}}{w_{11}+w_{01}} = \frac{5}{5+10} = \frac{1}{3}$ .

Depending on the gradient smoothness of the probabilistic black box, these explanations may slightly differ. However, if the additional six data points are placed such that the average black-box predictions of  $\mathcal{W}_{11} \cup \mathcal{W}_{10}$  and  $\mathcal{W}_{11} \cup \mathcal{W}_{01}$  are identical for both discretisations, the resulting explanations will be the same. Alternatively, if they are class predictions instead of probabilities, the two explanations will also be indistinguishable regardless of where the additional six instances are situated within their respective hyper-rectangles. The added benefit of this observation is evidence that partitioning each numerical feature into more than three splits is not beneficial, with the most important bin boundaries being the ones enclosing the explained data point.
